# Supplementary material for: Risk-Constrained Thompson Sampling for CVaR Bandits
Source: arXiv:2011.08046 source file (2021-02-04)
Supplement: Supplementary file 1 [file tau_conditions.tex]

\begin{center}
\textbf{\large Supplementary Material}
\end{center}

\section{Proof of Lemma~\ref{lem: tau_conditions}}
\label{sec: S-0}

\begin{proof}[Proof of Theorem~\ref{lem: tau_conditions}]

We prove by cases.
\begin{enumerate}
		\item We prove by contrapositive. Suppose on the contrary for all $\delta > 0$ there exists $\eeps \in (0,\delta)$ such that $\tau_\eeps(\alpha,\tau) \geq \mu_i - \mu_1$. By the infeasibility of arm $i$, we have
	$$\CVaR{\alpha}{i} -\CVaR{\alpha}{1} + \eeps > \tau - \CVaR{\alpha}{1} + \eeps = \paren{\frac{\alpha}{1-\alpha} + c_\alpha^*}\tau_\eeps(\alpha,\tau) \geq \paren{\frac{\alpha}{1-\alpha}} (\mu_i - \mu_1).$$
	By algebraic simplification,
	$$\CVaR{\alpha}{i} -\CVaR{\alpha}{1} + \eeps >  \CVaR{\alpha}{i} - \CVaR{\alpha}{1}  - c_\alpha^*(\sigma_i-\sigma_1) .$$
	Thus,
	$$\delta > \eeps >  c_\alpha^*( - (\sigma_i-\sigma_1)) = -c_\alpha^*(\sigma_i-\sigma_1).$$
	Since this holds for all $\delta > 0$, we have $-c_\alpha^*(\sigma_i-\sigma_1) \leq 0 \To \sigma_i \geq \sigma_1$.
	\item We prove by contrapositive. Suppose on the contrary for all $\delta > 0$ there exists $\eeps \in (0,\delta)$ such that $\tau_\eeps(\alpha,\tau) \geq \mu_i - \mu_1$. By the infeasibility of arm $i$, we have
	$$\CVaR{\alpha}{i} -\CVaR{\alpha}{1} + \eeps > \tau - \CVaR{\alpha}{1} + \eeps \geq \paren{\frac{\alpha}{1-\alpha} + c_\alpha^*}\tau_\eeps(\alpha,\tau) \geq \paren{\frac{\alpha}{1-\alpha}} (\mu_i - \mu_1) + c_\alpha^*(\mu_i - \mu_1).$$
	By algebraic simplification,
	$$\CVaR{\alpha}{i} -\CVaR{\alpha}{1} + \eeps >  \CVaR{\alpha}{i} - \CVaR{\alpha}{1}  - c_\alpha^*(\sigma_i-\sigma_1) + c_\alpha^*(\mu_i - \mu_1).$$
	Thus,
	$$\delta > \eeps >  c_\alpha^*(\mu_i - \mu_1 - (\sigma_i-\sigma_1)).$$
	Since this holds for all $\delta > 0$, we have $c_\alpha^*(\mu_i - \mu_1 - (\sigma_i-\sigma_1)) \leq 0 \To \mu_i - \mu_1 \leq \sigma_i - \sigma_1$.
	\item Suppose $\sigma_i - \sigma_1 \geq 0$ and $0 \leq (\tau - \CVaR{\alpha}{1})(1-\alpha)/\alpha < \mu_i - \mu_1 \leq \sigma_i - \sigma_1$ without loss of generality. Then 
	\begin{align*}
	(\CVaR{\alpha}{i} - \tau) - (\sigma_i - \sigma_1)c_\alpha^*
	&= 	\mu_i \paren{\frac{\alpha}{1-\alpha}} - \tau + \sigma_1 c_\alpha^*\\
	&= (\mu_i-\mu_1) \paren{\frac{\alpha}{1-\alpha}} +\CVaR{\alpha}{1} - \tau\\
	&> (\tau - \CVaR{\alpha}{1})\paren{\frac{1-\alpha}{\alpha}} \paren{\frac{\alpha}{1-\alpha}} +\CVaR{\alpha}{1} - \tau = 0.
	\end{align*}
	Choose $\delta = (\CVaR{\alpha}{i} - \tau) - (\sigma_i - \sigma_1)c_\alpha^*$. Then for $\eeps \in (0,\delta)$, we have
	\begin{align*}
	\tau_\eeps(\alpha,\tau)
	= \tau_0(\alpha,\tau+\eeps) &<  \frac{\tau - \CVaR{\alpha}{1} + (\CVaR{\alpha}{i} - \tau) - (\sigma_i - \sigma_1)c_\alpha^*}{{\alpha}/{(1-\alpha)} + c_\alpha^*}\\
	&< \frac{\CVaR{\alpha}{i} - \CVaR{\alpha}{1} - (\sigma_i - \sigma_1) c_\alpha^*}{{\alpha}/{(1-\alpha)} }\\
	&= \frac{(\mu_i - \mu_1) (\alpha/(1-\alpha))}{{\alpha}/{(1-\alpha)}} = \mu_i - \mu_1.
	\end{align*}
	\end{enumerate}

It follows that for any threshold level $\tau$ and feasible instance $(\nu,\tau)$, there exists $\alpha_0$ sufficiently close to $1$ such that for $\alpha \in (\alpha_0,1)$, there is a corresponding feasible instance $(\nu',\tau)$ such that for all infeasible arms $i \in \sdiff{[K]}{\kay_\tau}$, at least one of the three conditions are satisfied. Hence, $\tau_\eeps(\alpha,\tau) < \mu_i - \mu_1$.
\end{proof}
