# Supplementary material for: Risk-Constrained Thompson Sampling for CVaR Bandits
Source: arXiv:2011.08046 source file (2021-02-04)
Supplement: Supplementary file 11 [file supplementary.tex]

Various analyses of MABs involving risk measures have been undertaken.
\citet{sani2013riskaversion} considered \emph{mean-variance} as their risk measure, of bandits where the distribution of each arm $i$ has mean $\mu_i \in [0,1]$ and variance $\sigma_i^2 \in [0,1]$ respectively, and provided an LCB-based algorithm for regret analysis.
\citet{galichet2014exploration} provided the Multi-Armed Risk-Aware Bandit (\textsc{MaRaB}) algorithm with the objective of minimising the number of pulls of risky arms, using CVaR as their risk measure.
\citet{kyn2020cvar} similarly used CVaR as their risk measure and proposed the CVaR-UCB Algorithm, which chooses the arm with the highest gap from the arm with the highest CVaR. This happens since the authors consider the highest CVaR to result in highest reward, while our paper considers the highest CVaR to result in the highest cost. Thus, the discussions in that paper apply analogously.

\citet{kagrecha2020constrained} views a large CVaR to correspond to a larger loss incurred by the user and implemented RC-LCB. They considered the scenario where users have a predetermined risk tolerance level $\tau$, and any arm whose CVaR exceeds $\tau$ is deemed infeasible. This motivates the authors to define three different regrets, each corresponding to the number of times the non-optimal arms of varying natures were pulled. This problem formulation also includes that of \citet{kyn2020cvar} in the `infeasible instance' case. Having drawn inspiration from them in terms of the problem setup as well as the algorithm formulation, we will give proper definitions of these arms later which were originally defined in their paper.
\citet{zhu2020thompson} provided a Thomson sampling-based algorithm for the scenario in \citet{sani2013riskaversion}, where the arms follow Gaussian distributions with means and variances in their natural domains. Our paper draws inspiration from their formulation of the algorithm as well as their proofs for the various regret bounds.
